# Supplementary material for: Sentence Analogies: Exploring Linguistic Relationships and Regularities in Sentence Embeddings
Source: arXiv:2003.04036 source file (2020-03-09)
Supplement: Supplementary file 1 [file appendix.tex]

\appendix
\section{Experiment Results on Compositional Semantics Experiment}
\subsubsection{Negation Detection.}
% The results on Negation Detection are given in Fig.~\ref{fig:negation_detection}.
In Fig.~\ref{fig:negation_detection}, we observe that the InferSent model excels at recognizing negated sentences in comparison with other models, presumably due to the importance of detecting negation in NLI. One interesting finding is that the accuracy of the BERT Base model on this dataset surpasses that of the BERT Large model. Thus, increasing the depth of the model and the size of the training corpus does not necessarily make BERT better at distinguishing negation. ELMo does not fare well at detecting negation, but still outperforms the simple averaging of GloVe word embeddings.

\subsubsection{Negation Variants.}
Fig.~\ref{fig:negation_variant} assesses a separate form of negation involving quantifiers \cite{zhu2018exploring}.
Again, InferSent appears to obtain a much better understanding of negation quantifiers than other sentence embedding methods, owing to the importance of negation for NLI. BERT does not do well in terms of the accuracy, but it still outperforms Skip-Thought Vectors, ELMo, and word vector averaging. We conjecture that large-scale cloze task supervision may require a more focused understanding of negation semantics than needed for Skip-Thought Vectors or ELMo.

\begin{figure}[htbp]
\centering
\includegraphics[width=12cm]{figures/negation_detection.png}
\caption{Results for Negation Detection}
\label{fig:negation_detection}
\end{figure}

\begin{figure}[htbp]
\centering
\includegraphics[width=12cm]{figures/negation_variant.png}
\caption{Results for Negation Variants}
\vspace*{-4mm}
\label{fig:negation_variant}
\end{figure}

\begin{figure}[htbp]
\centering
\includegraphics[width=12cm]{figures/argument_sensitivity.png}
\caption{Results for Argument Sensitivity}
\label{fig:argument_sensitivity}
\end{figure}

%Considering the  negation detection and negation variants experiments together, we can conclude that supervised training on small natural language inference datasets is beneficial in enabling sentence representations encode negation in comparison with unsupervised learning on large corpus.
%In particular, increasing the size of the training corpus and the depth of the model does not help BERT in this scenario.
%lot in
%understanding negation related semantics.

\subsubsection{Argument Sensitivity.}
Fig.~\ref{fig:argument_sensitivity} considers an assessment that requires recognizing whether the order of verb arguments has been inverted \cite{zhu2018exploring}.
We observe that none of the analyzed methods showed the ability to account for the argument order with an accuracy of more than around 13\%. Hence, the models fail to adequately reflect the who-did-what-to-whom aspect of the sentence semantics in their representational proximity. 
%distinguish the semantic information from structural information on this data. 

\section{Experiment Results on Sentence Analogy Experiment}
\paragraph*{Common Capital City}
As \ref{table:countries} shows, sentence embeddings using $c^0$ DCT coefficients of fasttext word embeddings achieved best performance. Average of Glove embeddings also performs better than sentence embedding models based on RNNs and Transformers. For transformer based models, CLS pooling of RoBERTa-base model's accuracy is higher than other models, including RoBERTa-large model, which indicates that more model parameters and larger training corpus will not definitely lead to better performance on sentence analogy task. XLNet-Large model using CLS pooling performs worst on capital country dataset, even more worse than its base model using average pooling. None of the sentence embedding methods work well under fair setting, given a sentence analogy pairs with the form $A:B :: C: ?$, they prefer return $D^*$ which is equal to C instead of correct answer D. 
\begin{table}[htb]
\caption { Experiment results on Common Capital City sentence analogy pairs }
\centering
\begin{tabular}{|l|l|l|l|l|}
\hline
	 & 3CosADD Fair 	& 3CosADD  	& 3CosMul Fair 	 &3CosMul  \\ \hline
$c^0$ 	 & 0.4710 	 & 0.9899  	 & 0.6911  	 & 0.9673 	 \\ \hline
$c^{0:1}$ 	 & 0.2579 	 & 0.9827  	 & 0.5165  	 & 0.9585 	 \\ \hline
$c^{0:2}$ 	 & 0.1985 	 & 0.9604  	 & 0.3715  	 & 0.9052 	 \\ \hline
$c^{0:3}$ 	 & 0.1998 	 & 0.9712  	 & 0.3747  	 & 0.9349 	 \\ \hline
$c^{0:4}$ 	 & 0.1484 	 & 0.9606  	 & 0.3436  	 & 0.8603 	 \\ \hline
$c^{0:5}$ 	 & 0.1297 	 & 0.9593  	 & 0.3352  	 & 0.8740 	 \\ \hline
$c^{0:6}$ 	 & 0.1233 	 & 0.9760  	 & 0.3172  	 & 0.9308 	 \\ \hline
GLOVE-AVG 	 & 0.4200 	 & 0.9354  	 & 0.5178  	 & 0.9094 	 \\ \hline
BERT-BASE-AVG 	 & 0.2554 	 & 0.8527  	 & 0.3454  	 & 0.8675 	 \\ \hline
BERT-BASE-CLS 	 & 0.1042 	 & 0.1839  	 & 0.1053  	 & 0.1830 	 \\ \hline
BERT-LARGE-AVG 	 & 0.1513 	 & 0.8983  	 & 0.4797  	 & 0.8745 	 \\ \hline
BERT-LARGE-CLS 	 & 0.0753 	 & 0.0964  	 & 0.0748  	 & 0.0954 	 \\ \hline
GenSen 	 & 0.2240 	 & 0.6208  	 & 0.4060  	 & 0.4620 	 \\ \hline
InferSentV1 	 & 0.0780 	 & 0.7839  	 & 0.2297  	 & 0.7001 	 \\ \hline
InferSentV2 	 & 0.0738 	 & 0.9312  	 & 0.3948  	 & 0.6343 	 \\ \hline
QuickThought 	 & 0.0305 	 & 0.8335  	 & 0.1191  	 & 0.7707 	 \\ \hline
RoBERTa-BASE-AVG 	 & 0.2451 	 & 0.8694  	 & 0.2589  	 & 0.8687 	 \\ \hline
RoBERTa-BASE-CLS 	 & 0.1860 	 & 0.9144  	 & 0.1869  	 & 0.9143 	 \\ \hline
RoBERTa-LARGE-AVG 	 & 0.1224 	 & 0.7306  	 & 0.1237  	 & 0.7308 	 \\ \hline
RoBERTa-LARGE-CLS 	 & 0.0639 	 & 0.8008  	 & 0.0645  	 & 0.7998 	 \\ \hline
SkipThought 	 & 0.1613 	 & 0.6433  	 & 0.3643  	 & 0.5571 	 \\ \hline
UniversalSentenceDAN 	 & 0.0599 	 & 0.5769  	 & 0.1744  	 & 0.3886 	 \\ \hline
UniversalSentenceTransformer 	 & 0.2065 	 & 0.7780  	 & 0.3939  	 & 0.4943 	 \\ \hline
XLNet-BASE-AVG 	 & 0.0620 	 & 0.5153  	 & 0.0637  	 & 0.5175 	 \\ \hline
XLNet-BASE-CLS 	 & 0.0533 	 & 0.2154  	 & 0.0625  	 & 0.1995 	 \\ \hline
XLNet-LARGE-AVG 	 & 0.0208 	 & 0.1801  	 & 0.0212  	 & 0.1794 	 \\ \hline
XLNet-LARGE-CLS 	 & 0.0110 	 & 0.1322  	 & 0.0114  	 & 0.1312 	 \\ \hline
\end{tabular}
\label{table:countries}
\end{table}

\begin{table}[htb]
\caption { Experiment results on Common Capital City word analogy pairs }
\centering
\begin{tabular}{|l|l|l|l|l|}
\hline
	 & 3CosADD Fair 	& 3CosADD  	& 3CosMul Fair 	 &3CosMul  \\ \hline
GLOVE 	 & 0.4605 	 & 1.0000  	 & 0.8735  	 & 0.8755 	 \\ \hline
FastText 	 & 0.4802 	 & 1.0000  	 & 0.9802  	 & 0.9842 	 \\ \hline
BERT-BASE 	 & 0.3913 	 & 0.8992  	 & 0.5336  	 & 0.9111 	 \\ \hline
BERT-LARGE 	 & 0.0000 	 & 0.1028  	 & 0.0277  	 & 0.1285 	 \\ \hline
GenSen 	 & 0.6660 	 & 0.7490  	 & 0.6858  	 & 0.7510 	 \\ \hline
InferSentV1 	 & 0.4032 	 & 0.9486  	 & 0.8676  	 & 0.9526 	 \\ \hline
InferSentV2 	 & 0.4348 	 & 0.9881  	 & 0.6957  	 & 0.9901 	 \\ \hline
QuickThought 	 & 0.0000 	 & 0.8063  	 & 0.0079  	 & 0.8715 	 \\ \hline
RoBERTa-BASE 	 & 0.1383 	 & 0.5296  	 & 0.1383  	 & 0.5296 	 \\ \hline
RoBERTa-LARGE 	 & 0.0178 	 & 0.0237  	 & 0.0178  	 & 0.0237 	 \\ \hline
SkipThought 	 & 0.3834 	 & 0.7036  	 & 0.5652  	 & 0.7688 	 \\ \hline
UniversalSentenceDAN 	 & 0.1383 	 & 0.7134  	 & 0.5336  	 & 0.7549 	 \\ \hline
UniversalSentenceTransformer 	 & 0.6897 	 & 0.8735  	 & 0.7727  	 & 0.8182 	 \\ \hline
XLNet-BASE 	 & 0.0059 	 & 0.2905  	 & 0.0099  	 & 0.2846 	 \\ \hline
XLNet-LARGE 	 & 0.0000 	 & 0.2174  	 & 0.0000  	 & 0.2174 	 \\ \hline
\end{tabular}
\label{table:countries-word}
\end{table}

\paragraph*{All Capital Cities}
In table \ref{table:world}, we observe that $c^{0:1}$ performs better than other methods using 3CosADD metric in traditional settings while $c^{0:1}$ achieved best performance using 3CosMul on traditional settings. InferSent model trained on fasttext word embedding outperforms other RNNs or Transformer based models.  Transformer based models(like BERT, RoBERTa, XLNet) does not perform well on this dataset, partially because they use Byte Pair Encoding(BPE) tokenization. Although BPE tokenization reduces the size of vocabulary and number of out-of-vocabulary words, several country and capital words were tokenized into multiple sub words, which undermines the model's ability to capture relationship between sentences. 
\begin{table}[htb]
\caption { Experiment results on All Capital Cities sentence analogy pairs }
\centering
\begin{tabular}{|l|l|l|l|l|}
\hline
	 & 3CosADD Fair 	& 3CosADD  	& 3CosMul Fair 	 &3CosMul  \\ \hline
$c^0$ 	 & 0.3392 	 & 0.9674  	 & 0.5935  	 & 0.9266 	 \\ \hline
$c^{0:1}$ 	 & 0.2592 	 & 0.9727  	 & 0.4960  	 & 0.9188 	 \\ \hline
$c^{0:2}$ 	 & 0.1893 	 & 0.9551  	 & 0.3858  	 & 0.8746 	 \\ \hline
$c^{0:3}$ 	 & 0.1779 	 & 0.9339  	 & 0.3527  	 & 0.8274 	 \\ \hline
$c^{0:4}$ 	 & 0.1658 	 & 0.9541  	 & 0.3477  	 & 0.8675 	 \\ \hline
$c^{0:5}$ 	 & 0.1558 	 & 0.9036  	 & 0.3315  	 & 0.7249 	 \\ \hline
$c^{0:6}$ 	 & 0.1509 	 & 0.8716  	 & 0.3061  	 & 0.6243 	 \\ \hline
GLOVE-AVG 	 & 0.3302 	 & 0.8678  	 & 0.4852  	 & 0.8439 	 \\ \hline
BERT-BASE-AVG 	 & 0.0902 	 & 0.5085  	 & 0.1186  	 & 0.4934 	 \\ \hline
BERT-BASE-CLS 	 & 0.0325 	 & 0.0583  	 & 0.0327  	 & 0.0577 	 \\ \hline
BERT-LARGE-AVG 	 & 0.0925 	 & 0.5598  	 & 0.2385  	 & 0.4981 	 \\ \hline
BERT-LARGE-CLS 	 & 0.0171 	 & 0.0247  	 & 0.0172  	 & 0.0237 	 \\ \hline
GenSen 	 & 0.2105 	 & 0.4016  	 & 0.2779  	 & 0.3058 	 \\ \hline
InferSentV1 	 & 0.1048 	 & 0.7225  	 & 0.3081  	 & 0.6441 	 \\ \hline
InferSentV2 	 & 0.1065 	 & 0.9239  	 & 0.4401  	 & 0.6395 	 \\ \hline
QuickThought 	 & 0.0115 	 & 0.4529  	 & 0.0312  	 & 0.3524 	 \\ \hline
RoBERTa-BASE-AVG 	 & 0.0731 	 & 0.3838  	 & 0.0768  	 & 0.3812 	 \\ \hline
RoBERTa-BASE-CLS 	 & 0.0584 	 & 0.4627  	 & 0.0588  	 & 0.4626 	 \\ \hline
RoBERTa-LARGE-AVG 	 & 0.0465 	 & 0.4821  	 & 0.0469  	 & 0.4818 	 \\ \hline
RoBERTa-LARGE-CLS 	 & 0.0270 	 & 0.5140  	 & 0.0271  	 & 0.5136 	 \\ \hline
SkipThought 	 & 0.0844 	 & 0.4931  	 & 0.2197  	 & 0.4022 	 \\ \hline
UniversalSentenceDAN 	 & 0.0143 	 & 0.1517  	 & 0.0271  	 & 0.0549 	 \\ \hline
UniversalSentenceTransformer 	 & 0.1014 	 & 0.2980  	 & 0.0533  	 & 0.0763 	 \\ \hline
XLNet-BASE-AVG 	 & 0.0230 	 & 0.1588  	 & 0.0247  	 & 0.1582 	 \\ \hline
XLNet-BASE-CLS 	 & 0.0104 	 & 0.0719  	 & 0.0107  	 & 0.0299 	 \\ \hline
XLNet-LARGE-AVG 	 & 0.0065 	 & 0.0286  	 & 0.0065  	 & 0.0284 	 \\ \hline
XLNet-LARGE-CLS 	 & 0.0042 	 & 0.0148  	 & 0.0041  	 & 0.0140 	 \\ \hline
\end{tabular}
\label{table:world}
\end{table}

\begin{table}[htb]
\caption { Experiment results on All Capital Cities word analogy pairs }
\centering
\begin{tabular}{|l|l|l|l|l|}
\hline
    & 3CosADD Fair   & 3CosADD   & 3CosMul Fair     &3CosMul  \\ \hline
BERT-BASE    & 0.1529    & 0.3500    & 0.1996    & 0.3281    \\ \hline
BERT-LARGE   & 0.0031    & 0.0744    & 0.0226    & 0.0977    \\ \hline
FastText     & 0.3229    & 0.9912    & 0.8591    & 0.8830    \\ \hline
GLOVE     & 0.4250    & 0.9413    & 0.3175    & 0.3193    \\ \hline
GenSen    & 0.4858    & 0.5600    & 0.4922    & 0.5576    \\ \hline
InferSentV1     & 0.3639    & 0.8633    & 0.7217    & 0.8825    \\ \hline
InferSentV2     & 0.3119    & 0.9753    & 0.5479    & 0.9774    \\ \hline
QuickThought    & 0.0000    & 0.4618    & 0.0073    & 0.4810    \\ \hline
RoBERTa-BASE    & 0.0358    & 0.0936    & 0.0349    & 0.0921    \\ \hline
RoBERTa-LARGE   & 0.0034    & 0.0100    & 0.0035    & 0.0101    \\ \hline
SkipThought     & 0.2258    & 0.5955    & 0.4142    & 0.5991    \\ \hline
UniversalSentenceDAN     & 0.0251    & 0.1576    & 0.1178    & 0.1831    \\ \hline
UniversalSentenceTransformer   & 0.1694    & 0.2461    & 0.1965    & 0.2263    \\ \hline
XLNet-BASE   & 0.0031    & 0.0668    & 0.0037    & 0.0664    \\ \hline
XLNet-LARGE     & 0.0001    & 0.0340    & 0.0001    & 0.0343    \\ \hline
\end{tabular}
\label{table:world-word}
\end{table}

\paragraph*{City in State}
As table \ref{table:city} shows, all the sentence embedding model that we tested performed poor on city in state analogy dataset. It's probably due to the fact that most of the sentence embedding models we tested could not recognize the relationship between a state and city in that state.  
When asked with questions like:   
"They are going down to Arlington when they get cold: They are going down to Texas when they get cold :: There were no storms in Laredo in March: ?", 
Many sentence embedding models we will return a sentence containing a city name such as "There were no storms in Irving in March" instead of a sentence with a State name.  Table \ref{table:city-prob} shows the probability of different sentence embeddings returning a candidate sentence with a City name instead of State name. In a sentence embedding model get higher probability in table  \ref{table:city-prob}, it is less likely to recognize relationship between city and state. 

\begin{table}[htb]
\caption { Experiment results on city\_in\_state sentence analogy pairs }
\centering
\begin{tabular}{|l|l|l|l|l|}
\hline
	 & 3CosADD Fair 	& 3CosADD  	& 3CosMul Fair 	 &3CosMul  \\ \hline
$c^0$ 	 & 0.0677 	 & 0.2913  	 & 0.1139  	 & 0.2809 	 \\ \hline
$c^{0:1}$ 	 & 0.0589 	 & 0.2679  	 & 0.1059  	 & 0.2514 	 \\ \hline
$c^{0:2}$ 	 & 0.0444 	 & 0.2644  	 & 0.1207  	 & 0.2430 	 \\ \hline
$c^{0:3}$ 	 & 0.0294 	 & 0.2564  	 & 0.0821  	 & 0.2277 	 \\ \hline
$c^{0:4}$ 	 & 0.0263 	 & 0.2597  	 & 0.0834  	 & 0.2503 	 \\ \hline
$c^{0:5}$ 	 & 0.0241 	 & 0.2535  	 & 0.0725  	 & 0.2227 	 \\ \hline
$c^{0:6}$ 	 & 0.0222 	 & 0.2391  	 & 0.0556  	 & 0.2084 	 \\ \hline
GLOVE-AVG 	 & 0.0660 	 & 0.1559  	 & 0.0753  	 & 0.1503 	 \\ \hline
BERT-BASE-AVG 	 & 0.0258 	 & 0.1089  	 & 0.0341  	 & 0.1087 	 \\ \hline
BERT-BASE-CLS 	 & 0.0119 	 & 0.0128  	 & 0.0119  	 & 0.0127 	 \\ \hline
BERT-LARGE-AVG 	 & 0.0240 	 & 0.0832  	 & 0.0468  	 & 0.0795 	 \\ \hline
BERT-LARGE-CLS 	 & 0.0052 	 & 0.0058  	 & 0.0052  	 & 0.0057 	 \\ \hline
GenSen 	 & 0.0322 	 & 0.0672  	 & 0.0449  	 & 0.0497 	 \\ \hline
InferSentV1 	 & 0.0186 	 & 0.0935  	 & 0.0419  	 & 0.0806 	 \\ \hline
InferSentV2 	 & 0.0231 	 & 0.2054  	 & 0.0786  	 & 0.1421 	 \\ \hline
QuickThought 	 & 0.0089 	 & 0.0903  	 & 0.0203  	 & 0.0698 	 \\ \hline
RoBERTa-BASE-AVG 	 & 0.0304 	 & 0.0984  	 & 0.0318  	 & 0.0983 	 \\ \hline
RoBERTa-BASE-CLS 	 & 0.0289 	 & 0.1369  	 & 0.0290  	 & 0.1367 	 \\ \hline
RoBERTa-LARGE-AVG 	 & 0.0221 	 & 0.0896  	 & 0.0222  	 & 0.0896 	 \\ \hline
RoBERTa-LARGE-CLS 	 & 0.0187 	 & 0.1240  	 & 0.0187  	 & 0.1236 	 \\ \hline
SkipThought 	 & 0.0404 	 & 0.1589  	 & 0.0918  	 & 0.1167 	 \\ \hline
UniversalSentenceDAN 	 & 0.0128 	 & 0.0528  	 & 0.0293  	 & 0.0401 	 \\ \hline
UniversalSentenceTransformer 	 & 0.0439 	 & 0.1005  	 & 0.0493  	 & 0.0626 	 \\ \hline
XLNet-BASE-AVG 	 & 0.0120 	 & 0.0535  	 & 0.0128  	 & 0.0535 	 \\ \hline
XLNet-BASE-CLS 	 & 0.0060 	 & 0.0165  	 & 0.0071  	 & 0.0166 	 \\ \hline
XLNet-LARGE-AVG 	 & 0.0025 	 & 0.0106  	 & 0.0025  	 & 0.0104 	 \\ \hline
XLNet-LARGE-CLS 	 & 0.0020 	 & 0.0087  	 & 0.0017  	 & 0.0050 	 \\ \hline
\end{tabular}
\label{table:city}
\end{table}

\begin{table}[htb]
\caption { Probablity of sentence embeddings return city  on city\_in\_state dataset}
\centering
\begin{tabular}{|l|l|l|l|l|}
\hline
	 & 3CosADD Fair 	& 3CosADD  	& 3CosMul Fair 	 &3CosMul  \\ \hline
$c^0$ 	 & 0.8645 	 & 0.3061  	 & 0.7456  	 & 0.2838 	 \\ \hline
$c^{0:1}$ 	 & 0.8800 	 & 0.3622  	 & 0.7406  	 & 0.3423 	 \\ \hline
$c^{0:2}$ 	 & 0.9107 	 & 0.3896  	 & 0.7392  	 & 0.3811 	 \\ \hline
$c^{0:3}$ 	 & 0.9200 	 & 0.4313  	 & 0.7899  	 & 0.4291 	 \\ \hline
$c^{0:4}$ 	 & 0.9298 	 & 0.4434  	 & 0.8078  	 & 0.4228 	 \\ \hline
$c^{0:5}$ 	 & 0.9313 	 & 0.4539  	 & 0.7837  	 & 0.4482 	 \\ \hline
$c^{0:6}$ 	 & 0.9326 	 & 0.4973  	 & 0.8255  	 & 0.4989 	 \\ \hline
BERT-BASE-AVG 	 & 0.8763 	 & 0.5406  	 & 0.8303  	 & 0.4929 	 \\ \hline
BERT-BASE-CLS 	 & 0.6810 	 & 0.6545  	 & 0.6761  	 & 0.6500 	 \\ \hline
BERT-LARGE-AVG 	 & 0.8755 	 & 0.6412  	 & 0.6929  	 & 0.5183 	 \\ \hline
BERT-LARGE-CLS 	 & 0.7369 	 & 0.7132  	 & 0.7342  	 & 0.7134 	 \\ \hline
GLOVE-AVG 	 & 0.7289 	 & 0.4262  	 & 0.6610  	 & 0.3819 	 \\ \hline
GenSen 	 & 0.7134 	 & 0.5493  	 & 0.4491  	 & 0.4107 	 \\ \hline
InferSentV1 	 & 0.8319 	 & 0.5101  	 & 0.5892  	 & 0.3574 	 \\ \hline
InferSentV2 	 & 0.9207 	 & 0.4421  	 & 0.5610  	 & 0.3204 	 \\ \hline
QuickThought 	 & 0.8826 	 & 0.5106  	 & 0.6981  	 & 0.4292 	 \\ \hline
RoBERTa-BASE-AVG 	 & 0.8534 	 & 0.5974  	 & 0.8470  	 & 0.5910 	 \\ \hline
RoBERTa-BASE-CLS 	 & 0.8743 	 & 0.5461  	 & 0.8740  	 & 0.5457 	 \\ \hline
RoBERTa-LARGE-AVG 	 & 0.8939 	 & 0.6769  	 & 0.8936  	 & 0.6760 	 \\ \hline
RoBERTa-LARGE-CLS 	 & 0.9176 	 & 0.6418  	 & 0.9175  	 & 0.6418 	 \\ \hline
SkipThought 	 & 0.8559 	 & 0.5386  	 & 0.5068  	 & 0.3706 	 \\ \hline
UniversalSentenceDAN 	 & 0.8019 	 & 0.4815  	 & 0.4312  	 & 0.3236 	 \\ \hline
UniversalSentenceTransformer 	 & 0.7115 	 & 0.4595  	 & 0.3809  	 & 0.3067 	 \\ \hline
XLNet-BASE-AVG 	 & 0.8641 	 & 0.6691  	 & 0.8573  	 & 0.6609 	 \\ \hline
XLNet-BASE-CLS 	 & 0.8581 	 & 0.7620  	 & 0.8258  	 & 0.7314 	 \\ \hline
XLNet-LARGE-AVG 	 & 0.8533 	 & 0.7068  	 & 0.8523  	 & 0.7070 	 \\ \hline
XLNet-LARGE-CLS 	 & 0.7432 	 & 0.6224  	 & 0.6882  	 & 0.5908 	 \\ \hline\end{tabular}
\label{table:city-prob}
\end{table}

\begin{table}[htb]
\caption { Experiment results on city\_in\_state word analogy pairs }
\centering
\begin{tabular}{|l|l|l|l|l|}
\hline
    & 3CosADD Fair   & 3CosADD   & 3CosMul Fair     &3CosMul  \\ \hline
BERT-BASE    & 0.0213    & 0.0927    & 0.0459    & 0.1128    \\ \hline
BERT-LARGE   & 0.0041    & 0.0299    & 0.0072    & 0.0373    \\ \hline
FastText     & 0.0871    & 0.3790    & 0.3354    & 0.3763    \\ \hline
GLOVE     & 0.1364    & 0.2969    & 0.2429    & 0.2655    \\ \hline
GenSen    & 0.1011    & 0.1257    & 0.1024    & 0.1264    \\ \hline
InferSentV1     & 0.0767    & 0.1689    & 0.1746    & 0.2230    \\ \hline
InferSentV2     & 0.0683    & 0.3505    & 0.1346    & 0.3584    \\ \hline
QuickThought    & 0.0034    & 0.0710    & 0.0063    & 0.1063    \\ \hline
RoBERTa-BASE    & 0.0188    & 0.1027    & 0.0181    & 0.1018    \\ \hline
RoBERTa-LARGE   & 0.0127    & 0.0185    & 0.0127    & 0.0185    \\ \hline
SkipThought     & 0.1278    & 0.2474    & 0.1909    & 0.2562    \\ \hline
UniversalSentenceDAN     & 0.0208    & 0.0665    & 0.0468    & 0.0936    \\ \hline
UniversalSentenceTransformer   & 0.0699    & 0.1273    & 0.1056    & 0.1343    \\ \hline
XLNet-BASE   & 0.0059    & 0.0260    & 0.0066    & 0.0262    \\ \hline
XLNet-LARGE     & 0.0036    & 0.0145    & 0.0041    & 0.0152    \\ \hline
\end{tabular}
\end{table}

\paragraph*{Currency}
From table \ref{table: currency} and table \ref{table:currency-words}, we know that accuracy of all the sentence embedding models we tested are very low on currency analogy dataset under both fair and unfair settings. 
\begin{table}[htb]
\caption { Experiment results on currency sentence analogy pairs }
\centering
\begin{tabular}{|l|l|l|l|l|}
\hline
	 & 3CosADD Fair 	& 3CosADD  	& 3CosMul Fair 	 &3CosMul  \\ \hline
$c^0$ 	 & 0.0306 	 & 0.0663  	 & 0.0652  	 & 0.1029 	 \\ \hline
$c^{0:1}$ 	 & 0.0166 	 & 0.0536  	 & 0.0729  	 & 0.1037 	 \\ \hline
$c^{0:2}$ 	 & 0.0116 	 & 0.0437  	 & 0.0566  	 & 0.0892 	 \\ \hline
$c^{0:3}$ 	 & 0.0128 	 & 0.0438  	 & 0.0651  	 & 0.0887 	 \\ \hline
$c^{0:4}$ 	 & 0.0094 	 & 0.0369  	 & 0.0549  	 & 0.0770 	 \\ \hline
$c^{0:5}$ 	 & 0.0100 	 & 0.0341  	 & 0.0528  	 & 0.0651 	 \\ \hline
$c^{0:6}$ 	 & 0.0076 	 & 0.0312  	 & 0.0537  	 & 0.0634 	 \\ \hline
GLOVE-AVG 	 & 0.0211 	 & 0.0490  	 & 0.0308  	 & 0.0599 	 \\ \hline
BERT-BASE-AVG 	 & 0.0013 	 & 0.0082  	 & 0.0034  	 & 0.0102 	 \\ \hline
BERT-BASE-CLS 	 & 0.0085 	 & 0.0101  	 & 0.0086  	 & 0.0101 	 \\ \hline
BERT-LARGE-AVG 	 & 0.0014 	 & 0.0100  	 & 0.0289  	 & 0.0388 	 \\ \hline
BERT-LARGE-CLS 	 & 0.0062 	 & 0.0075  	 & 0.0043  	 & 0.0054 	 \\ \hline
GenSen 	 & 0.0006 	 & 0.0067  	 & 0.0075  	 & 0.0149 	 \\ \hline
InferSentV1 	 & 0.0006 	 & 0.0132  	 & 0.0038  	 & 0.0183 	 \\ \hline
InferSentV2 	 & 0.0023 	 & 0.0255  	 & 0.0432  	 & 0.0653 	 \\ \hline
QuickThought 	 & 0.0021 	 & 0.0094  	 & 0.0109  	 & 0.0169 	 \\ \hline
RoBERTa-BASE-AVG 	 & 0.0013 	 & 0.0068  	 & 0.0014  	 & 0.0070 	 \\ \hline
RoBERTa-BASE-CLS 	 & 0.0041 	 & 0.0125  	 & 0.0042  	 & 0.0126 	 \\ \hline
RoBERTa-LARGE-AVG 	 & 0.0010 	 & 0.0081  	 & 0.0010  	 & 0.0081 	 \\ \hline
RoBERTa-LARGE-CLS 	 & 0.0042 	 & 0.0099  	 & 0.0041  	 & 0.0099 	 \\ \hline
SkipThought 	 & 0.0007 	 & 0.0095  	 & 0.0075  	 & 0.0182 	 \\ \hline
UniversalSentenceDAN 	 & 0.0175 	 & 0.0344  	 & 0.0304  	 & 0.0369 	 \\ \hline
UniversalSentenceTransformer 	 & 0.0333 	 & 0.0438  	 & 0.0419  	 & 0.0460 	 \\ \hline
XLNet-BASE-AVG 	 & 0.0005 	 & 0.0055  	 & 0.0006  	 & 0.0053 	 \\ \hline
XLNet-BASE-CLS 	 & 0.0007 	 & 0.0043  	 & 0.0007  	 & 0.0042 	 \\ \hline
XLNet-LARGE-AVG 	 & 0.0011 	 & 0.0049  	 & 0.0011  	 & 0.0050 	 \\ \hline
XLNet-LARGE-CLS 	 & 0.0009 	 & 0.0034  	 & 0.0035  	 & 0.0053 	 \\ \hline
\end{tabular}
\label{table: currency}
\end{table}

\begin{table}[htb]
\caption { Experiment results on currency word analogy pairs }
\centering
\begin{tabular}{|l|l|l|l|l|}
\hline
    & 3CosADD Fair   & 3CosADD   & 3CosMul Fair     &3CosMul  \\ \hline
BERT-BASE    & 0.0023    & 0.0322    & 0.0011    & 0.0391    \\ \hline
BERT-LARGE   & 0.0023    & 0.0218    & 0.0057    & 0.0333    \\ \hline
FastText     & 0.2391    & 0.4736    & 0.3207    & 0.3253    \\ \hline
GLOVE     & 0.1356    & 0.2793    & 0.1402    & 0.1333    \\ \hline
GenSen    & 0.0069    & 0.0368    & 0.0115    & 0.0402    \\ \hline
InferSentV1     & 0.0816    & 0.1862    & 0.2080    & 0.3057    \\ \hline
InferSentV2     & 0.2000    & 0.3402    & 0.3023    & 0.4092    \\ \hline
QuickThought    & 0.0023    & 0.0460    & 0.0379    & 0.0782    \\ \hline
RoBERTa-BASE    & 0.0034    & 0.0161    & 0.0023    & 0.0149    \\ \hline
RoBERTa-LARGE   & 0.0034    & 0.0207    & 0.0046    & 0.0218    \\ \hline
SkipThought     & 0.0057    & 0.0977    & 0.0920    & 0.1655    \\ \hline
UniversalSentenceDAN     & 0.0103    & 0.0609    & 0.0701    & 0.0943    \\ \hline
UniversalSentenceTransformer   & 0.0598    & 0.0885    & 0.0862    & 0.1046    \\ \hline
XLNet-BASE   & 0.0011    & 0.0207    & 0.0011    & 0.0218    \\ \hline
XLNet-LARGE     & 0.0034    & 0.0460    & 0.0046    & 0.0460    \\ \hline
\end{tabular}
\label{table:currency-words}
\end{table}

\paragraph*{Man Woman}
In table \ref{table: family}, we observe that the DCT model excels at recognizing analogies between family comparison with other models.  Average of Glove word vectors also outperforms other more complicated models. By comparing  table \ref{table: family} and table \ref{table: family-words} We find that BERT and RoBERTa performs better in much better on sentence analogy tasks compared with word analogy tasks, which indicates that BERT based model works much better to capture analogy in long sentence than words. They are not suit to be directly used as word embeddings without context.

\begin{table}[htb]
\caption { Experiment results on Man Woman sentence analogy pairs }
\centering
\begin{tabular}{|l|l|l|l|l|}
\hline
	 & 3CosADD Fair 	& 3CosADD  	& 3CosMul Fair 	 &3CosMul  \\ \hline
$c^0$ 	 & 0.3815 	 & 0.9290  	 & 0.5589  	 & 0.9148 	 \\ \hline
$c^{0:1}$ 	 & 0.3228 	 & 0.9619  	 & 0.5691  	 & 0.9300 	 \\ \hline
$c^{0:2}$ 	 & 0.2622 	 & 0.9663  	 & 0.4621  	 & 0.9211 	 \\ \hline
$c^{0:3}$ 	 & 0.2252 	 & 0.9488  	 & 0.4717  	 & 0.9347 	 \\ \hline
$c^{0:4}$ 	 & 0.2054 	 & 0.8978  	 & 0.4710  	 & 0.8090 	 \\ \hline
$c^{0:5}$ 	 & 0.1712 	 & 0.8416  	 & 0.4049  	 & 0.7643 	 \\ \hline
$c^{0:6}$ 	 & 0.1557 	 & 0.8714  	 & 0.3578  	 & 0.8591 	 \\ \hline
GLOVE-AVG 	 & 0.4846 	 & 0.8778  	 & 0.5808  	 & 0.8648 	 \\ \hline
BERT-BASE-AVG 	 & 0.3971 	 & 0.7637  	 & 0.4849  	 & 0.7719 	 \\ \hline
BERT-BASE-CLS 	 & 0.2084 	 & 0.3514  	 & 0.2110  	 & 0.3496 	 \\ \hline
BERT-LARGE-AVG 	 & 0.2067 	 & 0.7065  	 & 0.4746  	 & 0.6650 	 \\ \hline
BERT-LARGE-CLS 	 & 0.0879 	 & 0.1904  	 & 0.0900  	 & 0.1867 	 \\ \hline
GenSen 	 & 0.0589 	 & 0.2871  	 & 0.0959  	 & 0.1474 	 \\ \hline
InferSentV1 	 & 0.3982 	 & 0.8179  	 & 0.6330  	 & 0.8305 	 \\ \hline
InferSentV2 	 & 0.4949 	 & 0.8737  	 & 0.3787  	 & 0.4283 	 \\ \hline
QuickThought 	 & 0.2982 	 & 0.5286  	 & 0.4453  	 & 0.5396 	 \\ \hline
RoBERTa-BASE-AVG 	 & 0.2192 	 & 0.7664  	 & 0.2319  	 & 0.7641 	 \\ \hline
RoBERTa-BASE-CLS 	 & 0.4403 	 & 0.7716  	 & 0.4408  	 & 0.7716 	 \\ \hline
RoBERTa-LARGE-AVG 	 & 0.1860 	 & 0.6559  	 & 0.1870  	 & 0.6557 	 \\ \hline
RoBERTa-LARGE-CLS 	 & 0.0752 	 & 0.5456  	 & 0.0754  	 & 0.5450 	 \\ \hline
SkipThought 	 & 0.2221 	 & 0.6607  	 & 0.4961  	 & 0.5906 	 \\ \hline
UniversalSentenceDAN 	 & 0.2487 	 & 0.4741  	 & 0.1609  	 & 0.2081 	 \\ \hline
UniversalSentenceTransformer 	 & 0.5255 	 & 0.6688  	 & 0.2498  	 & 0.2794 	 \\ \hline
XLNet-BASE-AVG 	 & 0.0759 	 & 0.5378  	 & 0.0807  	 & 0.5352 	 \\ \hline
XLNet-BASE-CLS 	 & 0.0377 	 & 0.3872  	 & 0.0514  	 & 0.3541 	 \\ \hline
XLNet-LARGE-AVG 	 & 0.0154 	 & 0.2996  	 & 0.0156  	 & 0.2984 	 \\ \hline
XLNet-LARGE-CLS 	 & 0.0084 	 & 0.2400  	 & 0.0091  	 & 0.2321 	 \\ \hline
\end{tabular}
\label{table: family}
\end{table} 

\begin{table}[htb]
\caption { Experiment results on Man Woman word analogy pairs }
\centering
\begin{tabular}{|l|l|l|l|l|}
\hline
    & 3CosADD Fair   & 3CosADD   & 3CosMul Fair     &3CosMul  \\ \hline
BERT-BASE    & 0.0405    & 0.6738    & 0.0500    & 0.6476    \\ \hline
BERT-LARGE   & 0.0024    & 0.3095    & 0.0048    & 0.3405    \\ \hline
FastText     & 0.2738    & 0.9952    & 0.7476    & 0.9524    \\ \hline
GLOVE     & 0.4500    & 0.9619    & 0.7452    & 0.8429    \\ \hline
GenSen    & 0.0167    & 0.4238    & 0.1310    & 0.5071    \\ \hline
InferSentV1     & 0.5667    & 0.9238    & 0.8381    & 0.9405    \\ \hline
InferSentV2     & 0.6881    & 0.9429    & 0.7786    & 0.9381    \\ \hline
QuickThought    & 0.2452    & 0.5619    & 0.5714    & 0.6952    \\ \hline
RoBERTa-BASE    & 0.0452    & 0.3595    & 0.0452    & 0.3595    \\ \hline
RoBERTa-LARGE   & 0.0143    & 0.1095    & 0.0143    & 0.1095    \\ \hline
SkipThought     & 0.2167    & 0.7690    & 0.6643    & 0.8262    \\ \hline
UniversalSentenceDAN     & 0.2429    & 0.7881    & 0.5810    & 0.7667    \\ \hline
UniversalSentenceTransformer   & 0.4238    & 0.8524    & 0.6881    & 0.8214    \\ \hline
XLNet-BASE   & 0.0095    & 0.3310    & 0.0095    & 0.3286    \\ \hline
XLNet-LARGE     & 0.0000    & 0.2619    & 0.0000    & 0.2643    \\ \hline
\end{tabular}
\label{table: family-words}
\end{table}

\paragraph*{Comparative}
As table \ref{table:comparative} shows, quick thought achieved state of the art performance on comparative analogy under traditional setting, while $c^{0}$ performs much better than other sentence embedding methods using 3CosMul function under fair settings. By comparing DCT embeddings with different K, we know that increasing K has negative effect on  model's accuracy on comparative analogy task.  Another interesting finding is that average pooling of BERT base model surpasses BERT large and RoBERTa, it seems that BERT model can not learn relationship between a sentence and its comparative form. CLS pooling of XLNet large model achieved lowest accuracy on this task, which indicates that Auto Regressive Transformer model is not good at capture comparative relationship.

\begin{table}[htb]
\caption { Experiment results on comparative sentence analogy pairs }
\centering
\begin{tabular}{|l|l|l|l|l|}
\hline
	 & 3CosADD Fair 	& 3CosADD  	& 3CosMul Fair 	 &3CosMul  \\ \hline
$c^0$ 	 & 0.3312 	 & 0.8861  	 & 0.5847  	 & 0.8844 	 \\ \hline
$c^{0:1}$ 	 & 0.0914 	 & 0.8501  	 & 0.4352  	 & 0.8585 	 \\ \hline
$c^{0:2}$ 	 & 0.0298 	 & 0.7671  	 & 0.3466  	 & 0.7993 	 \\ \hline
$c^{0:3}$ 	 & 0.0101 	 & 0.5955  	 & 0.2141  	 & 0.6420 	 \\ \hline
$c^{0:4}$ 	 & 0.0039 	 & 0.4305  	 & 0.1392  	 & 0.4957 	 \\ \hline
$c^{0:5}$ 	 & 0.0017 	 & 0.3138  	 & 0.0941  	 & 0.4035 	 \\ \hline
$c^{0:6}$ 	 & 0.0008 	 & 0.2428  	 & 0.0703  	 & 0.3378 	 \\ \hline
GLOVE-AVG 	 & 0.2145 	 & 0.8573  	 & 0.3370  	 & 0.8448 	 \\ \hline
BERT-BASE-AVG 	 & 0.1526 	 & 0.7877  	 & 0.2610  	 & 0.7912 	 \\ \hline
BERT-BASE-CLS 	 & 0.1109 	 & 0.2991  	 & 0.1135  	 & 0.2947 	 \\ \hline
BERT-LARGE-AVG 	 & 0.1330 	 & 0.7489  	 & 0.2919  	 & 0.4798 	 \\ \hline
BERT-LARGE-CLS 	 & 0.0364 	 & 0.0807  	 & 0.0354  	 & 0.0698 	 \\ \hline
GenSen 	 & 0.0423 	 & 0.7355  	 & 0.6704  	 & 0.8374 	 \\ \hline
InferSentV1 	 & 0.1266 	 & 0.8326  	 & 0.3022  	 & 0.7575 	 \\ \hline
InferSentV2 	 & 0.3217 	 & 0.8558  	 & 0.1662  	 & 0.1797 	 \\ \hline
QuickThought 	 & 0.0082 	 & 0.8903  	 & 0.1180  	 & 0.9019 	 \\ \hline
RoBERTa-BASE-AVG 	 & 0.3330 	 & 0.7143  	 & 0.3519  	 & 0.7145 	 \\ \hline
RoBERTa-BASE-CLS 	 & 0.0291 	 & 0.6291  	 & 0.0293  	 & 0.6290 	 \\ \hline
RoBERTa-LARGE-AVG 	 & 0.1473 	 & 0.7123  	 & 0.1498  	 & 0.7128 	 \\ \hline
RoBERTa-LARGE-CLS 	 & 0.0394 	 & 0.3301  	 & 0.0396  	 & 0.3293 	 \\ \hline
SkipThought 	 & 0.0037 	 & 0.7176  	 & 0.1283  	 & 0.5777 	 \\ \hline
UniversalSentenceDAN 	 & 0.0177 	 & 0.8174  	 & 0.0226  	 & 0.0546 	 \\ \hline
UniversalSentenceTransformer 	 & 0.0536 	 & 0.8429  	 & 0.0349  	 & 0.0610 	 \\ \hline
XLNet-BASE-AVG 	 & 0.0080 	 & 0.3568  	 & 0.0101  	 & 0.3588 	 \\ \hline
XLNet-BASE-CLS 	 & 0.0057 	 & 0.1595  	 & 0.0100  	 & 0.1001 	 \\ \hline
XLNet-LARGE-AVG 	 & 0.0031 	 & 0.1324  	 & 0.0033  	 & 0.1323 	 \\ \hline
XLNet-LARGE-CLS 	 & 0.0020 	 & 0.0744  	 & 0.0012  	 & 0.0610 	 \\ \hline
\end{tabular}
\label{table:comparative}
\end{table}

\begin{table}[htb]
\caption { Experiment results on comparative word analogy pairs }
\centering
\begin{tabular}{|l|l|l|l|l|}
\hline
    & 3CosADD Fair   & 3CosADD   & 3CosMul Fair     &3CosMul  \\ \hline
BERT-BASE    & 0.0469    & 0.3609    & 0.0908    & 0.3894    \\ \hline
BERT-LARGE   & 0.0077    & 0.1104    & 0.0169    & 0.1218    \\ \hline
FastText     & 0.4762    & 0.9472    & 0.6007    & 0.6094    \\ \hline
GLOVE     & 0.3559    & 0.8212    & 0.3113    & 0.3147    \\ \hline
GenSen    & 0.0342    & 0.5476    & 0.1771    & 0.6424    \\ \hline
InferSentV1     & 0.3123    & 0.8353    & 0.6850    & 0.8532    \\ \hline
InferSentV2     & 0.4425    & 0.9184    & 0.6778    & 0.9313    \\ \hline
QuickThought    & 0.0000    & 0.5789    & 0.0585    & 0.6696    \\ \hline
RoBERTa-BASE    & 0.1089    & 0.3802    & 0.1086    & 0.3805    \\ \hline
RoBERTa-LARGE   & 0.0387    & 0.0471    & 0.0379    & 0.0469    \\ \hline
SkipThought     & 0.0047    & 0.6508    & 0.5513    & 0.7130    \\ \hline
UniversalSentenceDAN     & 0.0072    & 0.5439    & 0.1128    & 0.5347    \\ \hline
UniversalSentenceTransformer   & 0.0702    & 0.7515    & 0.3100    & 0.7433    \\ \hline
XLNet-BASE   & 0.0122    & 0.1528    & 0.0146    & 0.1533    \\ \hline
XLNet-LARGE     & 0.0002    & 0.0918    & 0.0002    & 0.0925    \\ \hline
\end{tabular}
\label{table: comparative-words}
\end{table}

\paragraph*{Nationality Adjective}[htb]
Table \ref{table: nationality-adj} shows that $c^0$ achieves state-of-the-art performance on capturing analogy relationship between nationality and its corresponding adjective. InferSentV2 model transcends other RNNs based sentence embedding models. Besides that, we also notice that Universal Sentence Encoder model outperforms other Transformer based tasks like BERT, XLNet and RoBERTa since it uses supervised training data from SNLI.
Another interesting finding is that models that is good at capturing nationality adjective  analogy between words might fail on corresponding analogy questions between sentences. From table \ref{table: nationality-adj-words} and \ref{table: nationality-adj}, InferSent V1 and SkipThought model achieved high accuracy on word analogy question pairs, but their accuracy on sentence analogy are extremely low. 

\begin{table}[htb]
\caption { Experiment results on nationality\_adjective sentence analogy pairs }
\centering
\begin{tabular}{|l|l|l|l|l|}
\hline
	 & 3CosADD Fair 	& 3CosADD  	& 3CosMul Fair 	 &3CosMul  \\ \hline
$c^0$ 	 & 0.6317 	 & 0.8373  	 & 0.6403  	 & 0.8240 	 \\ \hline
$c^{0:1}$ 	 & 0.2223 	 & 0.3835  	 & 0.2655  	 & 0.4095 	 \\ \hline
$c^{0:2}$ 	 & 0.2377 	 & 0.3180  	 & 0.2676  	 & 0.3227 	 \\ \hline
$c^{0:3}$ 	 & 0.1171 	 & 0.1778  	 & 0.1330  	 & 0.1895 	 \\ \hline
$c^{0:4}$ 	 & 0.0387 	 & 0.0723  	 & 0.0484  	 & 0.0882 	 \\ \hline
$c^{0:5}$ 	 & 0.0370 	 & 0.0548  	 & 0.0407  	 & 0.0703 	 \\ \hline
$c^{0:6}$ 	 & 0.0386 	 & 0.0422  	 & 0.0407  	 & 0.0429 	 \\ \hline
GLOVE-AVG 	 & 0.4444 	 & 0.5544  	 & 0.4297  	 & 0.5192 	 \\ \hline
BERT-BASE-AVG 	 & 0.1754 	 & 0.3673  	 & 0.1938  	 & 0.3686 	 \\ \hline
BERT-BASE-CLS 	 & 0.0521 	 & 0.0641  	 & 0.0570  	 & 0.0681 	 \\ \hline
BERT-LARGE-AVG 	 & 0.1686 	 & 0.4743  	 & 0.2657  	 & 0.4658 	 \\ \hline
BERT-LARGE-CLS 	 & 0.0353 	 & 0.0455  	 & 0.0322  	 & 0.0343 	 \\ \hline
GenSen 	 & 0.0943 	 & 0.1109  	 & 0.1413  	 & 0.1541 	 \\ \hline
InferSentV1 	 & 0.1270 	 & 0.2942  	 & 0.1944  	 & 0.3372 	 \\ \hline
InferSentV2 	 & 0.2857 	 & 0.6834  	 & 0.5531  	 & 0.5630 	 \\ \hline
QuickThought 	 & 0.0389 	 & 0.3547  	 & 0.0794  	 & 0.3117 	 \\ \hline
RoBERTa-BASE-AVG 	 & 0.1972 	 & 0.2678  	 & 0.2033  	 & 0.2688 	 \\ \hline
RoBERTa-BASE-CLS 	 & 0.1400 	 & 0.3862  	 & 0.1401  	 & 0.3860 	 \\ \hline
RoBERTa-LARGE-AVG 	 & 0.0899 	 & 0.1320  	 & 0.0900  	 & 0.1321 	 \\ \hline
RoBERTa-LARGE-CLS 	 & 0.0907 	 & 0.1773  	 & 0.0908  	 & 0.1764 	 \\ \hline
SkipThought 	 & 0.0289 	 & 0.0665  	 & 0.0622  	 & 0.0934 	 \\ \hline
UniversalSentenceDAN 	 & 0.0585 	 & 0.4646  	 & 0.1072  	 & 0.1856 	 \\ \hline
UniversalSentenceTransformer 	 & 0.2328 	 & 0.5709  	 & 0.2142  	 & 0.2594 	 \\ \hline
XLNet-BASE-AVG 	 & 0.0451 	 & 0.0671  	 & 0.0458  	 & 0.0679 	 \\ \hline
XLNet-BASE-CLS 	 & 0.0302 	 & 0.0408  	 & 0.0355  	 & 0.0450 	 \\ \hline
XLNet-LARGE-AVG 	 & 0.0049 	 & 0.0120  	 & 0.0051  	 & 0.0121 	 \\ \hline
XLNet-LARGE-CLS 	 & 0.0039 	 & 0.0066  	 & 0.0052  	 & 0.0078 	 \\ \hline
\end{tabular}
\label{table: nationality-adj}
\end{table}

\begin{table}[htb]
\caption { Experiment results on nationality\_adjective word analogy pairs }
\centering
\begin{tabular}{|l|l|l|l|l|}
\hline
    & 3CosADD Fair   & 3CosADD   & 3CosMul Fair     &3CosMul  \\ \hline
BERT-BASE    & 0.2604    & 0.7183    & 0.3720    & 0.7250    \\ \hline
BERT-LARGE   & 0.0159    & 0.2854    & 0.0707    & 0.3140    \\ \hline
FastText     & 0.9244    & 0.9921    & 0.8476    & 0.8476    \\ \hline
GLOVE     & 0.8439    & 0.9555    & 0.5323    & 0.5305    \\ \hline
GenSen    & 0.6530    & 0.6732    & 0.6671    & 0.6860    \\ \hline
InferSentV1     & 0.7280    & 0.9134    & 0.9207    & 0.9427    \\ \hline
InferSentV2     & 0.9183    & 0.9787    & 0.9537    & 0.9774    \\ \hline
QuickThought    & 0.0073    & 0.6872    & 0.0671    & 0.7707    \\ \hline
RoBERTa-BASE    & 0.2835    & 0.5280    & 0.2829    & 0.5274    \\ \hline
RoBERTa-LARGE   & 0.0305    & 0.0829    & 0.0323    & 0.0841    \\ \hline
SkipThought     & 0.7213    & 0.8207    & 0.8409    & 0.8610    \\ \hline
UniversalSentenceDAN     & 0.3098    & 0.6445    & 0.5451    & 0.6713    \\ \hline
UniversalSentenceTransformer   & 0.6189    & 0.6823    & 0.6756    & 0.6902    \\ \hline
XLNet-BASE   & 0.0530    & 0.3213    & 0.0646    & 0.3250    \\ \hline
XLNet-LARGE     & 0.0012    & 0.2079    & 0.0018    & 0.2091    \\ \hline
\end{tabular}
\label{table: nationality-adj-words}
\end{table}

\paragraph*{Opposite}
From table \ref{table:opposite-words}, all the sentence embedding models excpet XLNet Large and CLS pooling of BERT large achieve relatively high accuracy on opposite analogy task under traditional setting, while average of Glove embeddings performs slightly better than other models. None of the models perform better than random guessing under fair settings. Given a sentence analogy question with the form $A: B :: C: D$, 3CosAdd metric finds sentence D by optimizing
\begin{equation}
    \argmax(\cos(D, C) + \cos(D, B) - \cos(D, A)) \label{eq:3cosADD}
\end{equation} 
We find that $ \cos(D, B) - \cos(D, A)$ is usually very small in our experiment, so equation \ref{eq:3cosADD} degenerates to $\argmax(\cos(D, C))$. Since $\cos(C, C) = 1$, all the sentence embedding models tends to return C instead of correct answer D under fair settings. This also applies to 3CosMul.
\begin{table}[htb]
\caption { Experiment Results on opposite sentence analogy pairs }
\centering
\begin{tabular}{|l|l|l|l|l|}
\hline
	 & 3CosADD Fair 	& 3CosADD  	& 3CosMul Fair 	 &3CosMul  \\ \hline
$c^0$ 	 & 0.2304 	 & 0.9010  	 & 0.3291  	 & 0.9073 	 \\ \hline
$c^{0:1}$ 	 & 0.1452 	 & 0.8933  	 & 0.2588  	 & 0.9007 	 \\ \hline
$c^{0:2}$ 	 & 0.1076 	 & 0.8963  	 & 0.2201  	 & 0.9032 	 \\ \hline
$c^{0:3}$ 	 & 0.0858 	 & 0.8913  	 & 0.1962  	 & 0.8965 	 \\ \hline
$c^{0:4}$ 	 & 0.0729 	 & 0.8926  	 & 0.1843  	 & 0.8989 	 \\ \hline
$c^{0:5}$ 	 & 0.0631 	 & 0.8909  	 & 0.1668  	 & 0.8968 	 \\ \hline
$c^{0:6}$ 	 & 0.0539 	 & 0.8896  	 & 0.1539  	 & 0.8955 	 \\ \hline
GLOVE-AVG 	 & 0.2582 	 & 0.9039  	 & 0.3122  	 & 0.9071 	 \\ \hline
BERT-BASE-AVG 	 & 0.0828 	 & 0.8885  	 & 0.1194  	 & 0.8914 	 \\ \hline
BERT-BASE-CLS 	 & 0.1294 	 & 0.6644  	 & 0.1345  	 & 0.6590 	 \\ \hline
BERT-LARGE-AVG 	 & 0.0446 	 & 0.8792  	 & 0.1468  	 & 0.7561 	 \\ \hline
BERT-LARGE-CLS 	 & 0.0876 	 & 0.2759  	 & 0.0864  	 & 0.2367 	 \\ \hline
QuickThought 	 & 0.0593 	 & 0.8841  	 & 0.2222  	 & 0.8860 	 \\ \hline
RoBERTa-BASE-AVG 	 & 0.0779 	 & 0.8937  	 & 0.0840  	 & 0.8941 	 \\ \hline
RoBERTa-BASE-CLS 	 & 0.0380 	 & 0.8817  	 & 0.0385  	 & 0.8817 	 \\ \hline
RoBERTa-LARGE-AVG 	 & 0.0434 	 & 0.8812  	 & 0.0442  	 & 0.8812 	 \\ \hline
RoBERTa-LARGE-CLS 	 & 0.0331 	 & 0.8230  	 & 0.0336  	 & 0.8221 	 \\ \hline
SkipThought 	 & 0.0345 	 & 0.8839  	 & 0.1181  	 & 0.5248 	 \\ \hline
UniversalSentenceDAN 	 & 0.0407 	 & 0.8780  	 & 0.0242  	 & 0.0609 	 \\ \hline
UniversalSentenceTransformer 	 & 0.1122 	 & 0.8816  	 & 0.0266  	 & 0.0489 	 \\ \hline
XLNet-BASE-AVG 	 & 0.0230 	 & 0.8678  	 & 0.0261  	 & 0.8675 	 \\ \hline
XLNet-BASE-CLS 	 & 0.0217 	 & 0.7836  	 & 0.0268  	 & 0.5678 	 \\ \hline
XLNet-LARGE-AVG 	 & 0.0175 	 & 0.6292  	 & 0.0181  	 & 0.6280 	 \\ \hline
XLNet-LARGE-CLS 	 & 0.0134 	 & 0.4511  	 & 0.0092  	 & 0.3241 	 \\ \hline
\end{tabular}
\label{table:opposite}
\end{table}

\begin{table}[htb]
\caption { Experiment results on opposite word analogy pairs }
\centering
\begin{tabular}{|l|l|l|l|l|}
\hline
    & 3CosADD Fair   & 3CosADD   & 3CosMul Fair     &3CosMul  \\ \hline
BERT-BASE    & 0.0000    & 0.1283    & 0.0017    & 0.1300    \\ \hline
BERT-LARGE   & 0.0017    & 0.1017    & 0.0100    & 0.1100    \\ \hline
FastText     & 0.0950    & 0.8083    & 0.5933    & 0.7683    \\ \hline
GLOVE     & 0.0983    & 0.6017    & 0.4333    & 0.5600    \\ \hline
GenSen    & 0.0017    & 0.4467    & 0.0767    & 0.6033    \\ \hline
InferSentV1     & 0.1850    & 0.4900    & 0.3783    & 0.5633    \\ \hline
InferSentV2     & 0.3250    & 0.5933    & 0.4533    & 0.6483    \\ \hline
QuickThought    & 0.0000    & 0.5700    & 0.1100    & 0.7350    \\ \hline
RoBERTa-BASE    & 0.0100    & 0.1850    & 0.0117    & 0.1850    \\ \hline
RoBERTa-LARGE   & 0.0167    & 0.0767    & 0.0150    & 0.0750    \\ \hline
SkipThought     & 0.0000    & 0.3833    & 0.1033    & 0.4617    \\ \hline
UniversalSentenceDAN     & 0.0000    & 0.6150    & 0.0600    & 0.5900    \\ \hline
UniversalSentenceTransformer   & 0.0450    & 0.7233    & 0.2567    & 0.7100    \\ \hline
XLNet-BASE   & 0.0000    & 0.1400    & 0.0033    & 0.1433    \\ \hline
XLNet-LARGE     & 0.0017    & 0.1000    & 0.0017    & 0.1017    \\ \hline
\end{tabular}
\label{table:opposite-words}
\end{table}

\paragraph*{Plural}
Table \ref{table:plural} exhibits that most of the sentence embedding models got very high accuracy under traditional settings, which means that they are capable of capturing morphology information in a sentence. But their experienced a sharp drop in performance when switching to fair settings.  By comparing accuracy of CLS pooling and average pooling of BERT based result, we can draw a conclusion that average pooling does better in recognizing relationship between a noun and its plural form.

\begin{table}[htb]
\caption { Experiment Results on plural sentence analogy pairs }
\centering
\begin{tabular}{|l|l|l|l|l|}
\hline
	 & 3CosADD Fair 	& 3CosADD  	& 3CosMul Fair 	 &3CosMul  \\ \hline
$c^0$ 	 & 0.3365 	 & 0.9872  	 & 0.5370  	 & 0.9875 	 \\ \hline
$c^{0:1}$ 	 & 0.1853 	 & 0.9876  	 & 0.4163  	 & 0.9881 	 \\ \hline
$c^{0:2}$ 	 & 0.1288 	 & 0.9882  	 & 0.3623  	 & 0.9882 	 \\ \hline
$c^{0:3}$ 	 & 0.0924 	 & 0.9881  	 & 0.3029  	 & 0.9875 	 \\ \hline
$c^{0:4}$ 	 & 0.0679 	 & 0.9886  	 & 0.2591  	 & 0.9882 	 \\ \hline
$c^{0:5}$ 	 & 0.0530 	 & 0.9883  	 & 0.2308  	 & 0.9882 	 \\ \hline
$c^{0:6}$ 	 & 0.0428 	 & 0.9870  	 & 0.2108  	 & 0.9876 	 \\ \hline
GLOVE-AVG 	 & 0.3318 	 & 0.9852  	 & 0.4319  	 & 0.9836 	 \\ \hline
BERT-BASE-AVG 	 & 0.1252 	 & 0.9871  	 & 0.1934  	 & 0.9875 	 \\ \hline
BERT-BASE-CLS 	 & 0.1577 	 & 0.7747  	 & 0.1648  	 & 0.7676 	 \\ \hline
BERT-LARGE-AVG 	 & 0.0880 	 & 0.9873  	 & 0.3223  	 & 0.9410 	 \\ \hline
BERT-LARGE-CLS 	 & 0.1205 	 & 0.4148  	 & 0.1158  	 & 0.3601 	 \\ \hline
GenSen 	 & 0.0374 	 & 0.9849  	 & 0.6000  	 & 0.9858 	 \\ \hline
InferSentV1 	 & 0.0908 	 & 0.9867  	 & 0.2515  	 & 0.9859 	 \\ \hline
InferSentV2 	 & 0.1285 	 & 0.9900  	 & 0.4236  	 & 0.7282 	 \\ \hline
QuickThought 	 & 0.0413 	 & 0.9817  	 & 0.2487  	 & 0.9846 	 \\ \hline
RoBERTa-BASE-AVG 	 & 0.2034 	 & 0.9862  	 & 0.2171  	 & 0.9862 	 \\ \hline
RoBERTa-BASE-CLS 	 & 0.1047 	 & 0.9833  	 & 0.1055  	 & 0.9833 	 \\ \hline
RoBERTa-LARGE-AVG 	 & 0.1368 	 & 0.9830  	 & 0.1388  	 & 0.9830 	 \\ \hline
RoBERTa-LARGE-CLS 	 & 0.0519 	 & 0.9235  	 & 0.0530  	 & 0.9228 	 \\ \hline
SkipThought 	 & 0.0280 	 & 0.9846  	 & 0.1476  	 & 0.6373 	 \\ \hline
UniversalSentenceDAN 	 & 0.0164 	 & 0.9835  	 & 0.0254  	 & 0.0793 	 \\ \hline
UniversalSentenceTransformer 	 & 0.1010 	 & 0.9845  	 & 0.0451  	 & 0.1146 	 \\ \hline
XLNet-BASE-AVG 	 & 0.0292 	 & 0.9786  	 & 0.0336  	 & 0.9780 	 \\ \hline
XLNet-BASE-CLS 	 & 0.0289 	 & 0.9052  	 & 0.0323  	 & 0.6363 	 \\ \hline
XLNet-LARGE-AVG 	 & 0.0264 	 & 0.7661  	 & 0.0273  	 & 0.7650 	 \\ \hline
XLNet-LARGE-CLS 	 & 0.0188 	 & 0.5650  	 & 0.0135  	 & 0.4650 	 \\ \hline
\end{tabular}
\label{table:plural}
\end{table}

\begin{table}[htb]
\caption { Experiment results on plural word analogy pairs }
\centering
\begin{tabular}{|l|l|l|l|l|}
\hline
    & 3CosADD Fair   & 3CosADD   & 3CosMul Fair     &3CosMul  \\ \hline
BERT-BASE    & 0.0198    & 0.8330    & 0.0525    & 0.8218    \\ \hline
BERT-LARGE   & 0.0022    & 0.4535    & 0.0107    & 0.4517    \\ \hline
FastText     & 0.0172    & 0.9692    & 0.1770    & 0.1954    \\ \hline
GLOVE     & 0.0226    & 0.9502    & 0.0944    & 0.1244    \\ \hline
GenSen    & 0.0756    & 0.7575    & 0.4704    & 0.8109    \\ \hline
InferSentV1     & 0.0068    & 0.9367    & 0.1503    & 0.9325    \\ \hline
InferSentV2     & 0.0186    & 0.9597    & 0.0735    & 0.9615    \\ \hline
QuickThought    & 0.0019    & 0.8237    & 0.0951    & 0.8137    \\ \hline
RoBERTa-BASE    & 0.1042    & 0.6487    & 0.1040    & 0.6481    \\ \hline
RoBERTa-LARGE   & 0.0308    & 0.1430    & 0.0312    & 0.1433    \\ \hline
SkipThought     & 0.0226    & 0.7120    & 0.2359    & 0.3287    \\ \hline
UniversalSentenceDAN     & 0.0030    & 0.7678    & 0.1561    & 0.5877    \\ \hline
UniversalSentenceTransformer   & 0.0629    & 0.8797    & 0.4274    & 0.7824    \\ \hline
XLNet-BASE   & 0.0190    & 0.4267    & 0.0215    & 0.4221    \\ \hline
XLNet-LARGE     & 0.0005    & 0.1316    & 0.0007    & 0.1315    \\ \hline
\end{tabular}
\end{table}

\paragraph*{Plural Verbs}
From table \ref{table: plural-verbs}, $c^{0:1}$ beats other models in recognizing plural form of verbs under both fair and traditional setting. Accuracy of DCT embeddings drops when increasing K. QuickThought Vector outperforms other RNNs and Transformer based models when using 3CosMul metric. Deep Average Network excels other sentence embedding models under traditional settings using 3CosADD but its performance drops drastically when switching to 3CosMul metric. CLS pooling of BERT and XLNet model
got very low accuracy on both settings, which indicates that CLS pooling is not able to capture morphology information in sentences.

\begin{table}[htb]
\caption { Experiment Results on plural\_verbs sentence analogy pairs }
\centering
\begin{tabular}{|l|l|l|l|l|}
\hline
	 & 3CosADD Fair 	& 3CosADD  	& 3CosMul Fair 	 &3CosMul  \\ \hline
$c^0$ 	 & 0.4547 	 & 0.9635  	 & 0.6913  	 & 0.9680 	 \\ \hline
$c^{0:1}$ 	 & 0.3554 	 & 0.9698  	 & 0.7033  	 & 0.9772 	 \\ \hline
$c^{0:2}$ 	 & 0.2101 	 & 0.9530  	 & 0.5815  	 & 0.9612 	 \\ \hline
$c^{0:3}$ 	 & 0.1267 	 & 0.9358  	 & 0.4835  	 & 0.9469 	 \\ \hline
$c^{0:4}$ 	 & 0.0792 	 & 0.9280  	 & 0.4072  	 & 0.9368 	 \\ \hline
$c^{0:5}$ 	 & 0.0499 	 & 0.9180  	 & 0.3427  	 & 0.9280 	 \\ \hline
$c^{0:6}$ 	 & 0.0316 	 & 0.9142  	 & 0.2945  	 & 0.9237 	 \\ \hline
GLOVE-AVG 	 & 0.4707 	 & 0.9032  	 & 0.5439  	 & 0.8844 	 \\ \hline
BERT-BASE-AVG 	 & 0.1651 	 & 0.8648  	 & 0.2423  	 & 0.8701 	 \\ \hline
BERT-BASE-CLS 	 & 0.1196 	 & 0.2702  	 & 0.1222  	 & 0.2655 	 \\ \hline
BERT-LARGE-AVG 	 & 0.0697 	 & 0.8741  	 & 0.3144  	 & 0.7978 	 \\ \hline
BERT-LARGE-CLS 	 & 0.0275 	 & 0.0674  	 & 0.0254  	 & 0.0512 	 \\ \hline
GenSen 	 & 0.1254 	 & 0.8507  	 & 0.5561  	 & 0.8911 	 \\ \hline
InferSentV1 	 & 0.2113 	 & 0.8264  	 & 0.3781  	 & 0.7867 	 \\ \hline
InferSentV2 	 & 0.3019 	 & 0.8267  	 & 0.2108  	 & 0.3220 	 \\ \hline
QuickThought 	 & 0.1497 	 & 0.8846  	 & 0.4149  	 & 0.9107 	 \\ \hline
RoBERTa-BASE-AVG 	 & 0.2262 	 & 0.9018  	 & 0.2418  	 & 0.9025 	 \\ \hline
RoBERTa-BASE-CLS 	 & 0.0859 	 & 0.8481  	 & 0.0865  	 & 0.8481 	 \\ \hline
RoBERTa-LARGE-AVG 	 & 0.1473 	 & 0.9087  	 & 0.1495  	 & 0.9088 	 \\ \hline
RoBERTa-LARGE-CLS 	 & 0.0939 	 & 0.7953  	 & 0.0945  	 & 0.7943 	 \\ \hline
SkipThought 	 & 0.0703 	 & 0.8393  	 & 0.2797  	 & 0.6175 	 \\ \hline
UniversalSentenceDAN 	 & 0.0615 	 & 0.9289  	 & 0.0492  	 & 0.0981 	 \\ \hline
UniversalSentenceTransformer 	 & 0.1851 	 & 0.9138  	 & 0.0355  	 & 0.0515 	 \\ \hline
XLNet-BASE-AVG 	 & 0.0117 	 & 0.7091  	 & 0.0134  	 & 0.7092 	 \\ \hline
XLNet-BASE-CLS 	 & 0.0078 	 & 0.4843  	 & 0.0145  	 & 0.3868 	 \\ \hline
XLNet-LARGE-AVG 	 & 0.0102 	 & 0.3173  	 & 0.0105  	 & 0.3162 	 \\ \hline
XLNet-LARGE-CLS 	 & 0.0078 	 & 0.2103  	 & 0.0062  	 & 0.1774 	 \\ \hline
\end{tabular}
\label{table: plural-verbs}
\end{table}

 \begin{table}[htb]
\caption { Experiment results on plural\_verbs word analogy pairs }
\centering
\begin{tabular}{|l|l|l|l|l|}
\hline
    & 3CosADD Fair   & 3CosADD   & 3CosMul Fair     &3CosMul  \\ \hline
BERT-BASE    & 0.0435    & 0.8735    & 0.0791    & 0.8794    \\ \hline
BERT-LARGE   & 0.0000    & 0.3399    & 0.0119    & 0.3538    \\ \hline
FastText     & 0.3439    & 0.9704    & 0.7411    & 0.7391    \\ \hline
GLOVE     & 0.2885    & 0.9150    & 0.5850    & 0.6225    \\ \hline
GenSen    & 0.0079    & 0.9447    & 0.1146    & 0.9565    \\ \hline
InferSentV1     & 0.1462    & 0.9032    & 0.5336    & 0.9269    \\ \hline
InferSentV2     & 0.3458    & 0.9901    & 0.5692    & 0.9881    \\ \hline
QuickThought    & 0.0020    & 0.9526    & 0.4447    & 0.9783    \\ \hline
RoBERTa-BASE    & 0.3261    & 0.9881    & 0.3261    & 0.9881    \\ \hline
RoBERTa-LARGE   & 0.0711    & 0.2510    & 0.0711    & 0.2510    \\ \hline
SkipThought     & 0.0099    & 0.9466    & 0.7332    & 0.8320    \\ \hline
UniversalSentenceDAN     & 0.0198    & 0.5336    & 0.1621    & 0.5277    \\ \hline
UniversalSentenceTransformer   & 0.1028    & 0.8518    & 0.4091    & 0.8182    \\ \hline
XLNet-BASE   & 0.0138    & 0.4565    & 0.0217    & 0.4605    \\ \hline
XLNet-LARGE     & 0.0099    & 0.2510    & 0.0099    & 0.2510    \\ \hline
\end{tabular}
\label{table: plural-verbs-words}
\end{table}
